# Supplementary material for: SinGAN: Learning a Generative Model from a Single Natural Image
Source: arXiv:1905.01164 source file (2019-09-04)
Supplement: Supplementary file 1 [file SM.tex]

\section{Additional Information}

\subsection{Optimization}
At each scale, the weights of the generator and discriminator are initialized to those from the previous trained scale (except for the coarsest scale or when changing the number of kernels, in which cases we use random initialization). We train each scale for 2000 iterations. In each iteration we alternate between 3 gradient steps for the generator and 3 gradient steps for the discriminator. We use the Adam optimizer \cite{kingma2014adam} with a learning rate of $0.0005$ (decreased by a factor of $0.1$ after $1600$ iterations) and momentum parameters $\beta_1=0.5, \beta_2=0.999$. The weight of the reconstruction loss is $\alpha = 10$, and the weight of the gradient penalty in the WGAN loss is $0.1$. Training takes about $30$ minutes on a 1080TI GPU for an image of size $256\times256$ pixels, and the generation at test time is well under one second per image.

\subsection{Boundary conditions and the effect of padding}
The type of padding used within SinGAN's generators highly influences the diversity among generated samples at the corners (the net learns to associate the image structures at the corners with the artificial edges caused by the padding). Figure~\ref{fig:padding} illustrates this effect by depicting the standard deviation among generated samples for each location in the image. %A fully convolutional net fed with spatial random noise cannot associate structures with specific locations in the image (a shift in the input noise will always cause a shift in the output). This is true, however, only away from the boundaries. When using zero padding, we create artificial edges at the borders, which the net \emph{can} learn to associate with the specific structures.
%can be used to enforce boundary conditions and control the amount of variability at the image's borders.
As can be seen, zero padding in each layer leads to very small variability at the corners. This effect is reduced when, instead of padding within the layers, we zero-pad the inputs to the generator (both image and noise) by half the net's receptive field from each side. This is our default setting for generating samples. Finally, if the input image is zero-padded this way while the input noise is padded by noise (\ie taken to be larger), then the effect is further reduced. %, but may sometimes cause artifacts at the boundaries.
We use this configuration for generating animations.

%This helps the generator identify the image borders, and thus serves as a fixed boundary condition for the generation process. Figure~\ref{fig:padding} shows the effect of this padding scheme. Using zero padding at each convolution layer decreases the variability of the generated image. Padding with noise (\ie producing $z^n$ of larger size) insert artifacts to the image. Initially zero padding the input instead (our final setting) helps to generate high quality images with nice structure variability. 

\begin{figure}[h!]
    \center
	\includegraphics[width=0.8\textwidth]{padding.pdf}
	\caption{\textbf{Effect of padding.} The padding configuration highly effects the diversity between samples at the corners. Zero padding in each convolutional layer (layer padding) leads to only minor variability at the corners. Padding only the input to the net (initial padding), leads to somewhat increased variability at the corners. Finally, padding by noise, leads to high variability.}
	\label{fig:padding}
\end{figure}

\begin{figure}[h!]
    \center
	\includegraphics[width=0.8\textwidth]{manipulation_scheme.pdf}
	\caption{\textbf{Image manipulation using SinGAN.} Once a SinGAN model is trained, we can inject an image to one of its coarser scales so as to match its patch distribution to that of the training image. In this example, we feed a downsampled version of a horse image (bottom left) into the $7$th scale of a $10$-scale SinGAN model that was trained on a Zebra image (bottom right). As the this input propagates through the generation pyramid, stripes are gradually added to the horse, which grant it the appearance of a Zebra.}
	\label{fig:manipulation_scheme}
\end{figure}

\subsection{Effect of the injection scale for image manipulation}
In all image manipulation tasks illustrated in the paper, we inject (a possibly downsampled version of) an image into the generation pyramid at some scale $n<N$, and feed forward %this input image in the following levels, 
it through the generators up to the finest scale. This paradigm is illustrated in Fig.~\ref{fig:manipulation_scheme}, where a SinGAN trained on a single Zebra image, adds stripes to a horse injected at a coarse scale. %, so as to match its patch distribution to that of the training image. 
Different injection scales lead to different effects. We demonstrate this in Fig.~\ref{fig:manipulation_scale} in the context of harmonization, paint-to-image, and image editing. As can be seen, the coarser the injection scale, the larger the structures that SinGAN can modify so as to match the statistics of patches in the generated to the training image. Injection at fine scales, only modifies small scale structures and textures, while leaving the global structure intact.

\begin{figure}
	\includegraphics[width=1\textwidth]{manipulation_scale.pdf}
	\caption{\textbf{Effect of the injection scale for image manipulation.} In applications such as harmonization (top), paint-to-image (middle), and editing (bottom), the coarser the scale we inject the input image, the larger the structures that get modified. When the input is injected at fine scales, only the fine textures get modified while the global structure remains fixed.}
	\label{fig:manipulation_scale}
	\vspace{10cm}
\end{figure}

\subsection{Animation from a single image}
To animate a single image $x$, we introduce smooth random changes to SinGAN's noise maps, while restricting them to remain close to the noise maps that generate $x$. Those perturbations produce images with similar layout, and thus create a sequence of images with gradually changed composition. Specifically, denoting by $z_n(t)$ the $n$th scale noise map at time $t$, we construct our random walk as
%\begin{eqnarray*}
%[z_n]_i= \left\{ 
%\begin{matrix}
%{z_n^{rec}} \quad &i=0\\ 
%\alpha z_n^{rec} + (1-\alpha)([z_n]_{i-1}+[z_n]_i^{\text{diff}})  \quad &i\geq 1 \\
%\end{matrix} \right 
%\\ 
%[z_n]_i^{\text{diff}} = \beta ([z_n]_{i-1}-[z_n]_{i-2})+ (1-\beta) z_n^{\text{rand}} 
%\end{eqnarray*}
\begin{align*}
z_n(t+1)&= \alpha z_n^{rec} + (1-\alpha)\left(z_n(t)+z_n^{\text{diff}}(t+1)\right), \nonumber\\
z_n^{\text{diff}}(t+1) &= \beta \left(z_n(t)-z_n(t-1)\right)+ (1-\beta) u_n(t) 
\end{align*}
where $z_n(0)=z_n^\text{rec}$ and $u_n(t)$ is a an iid sequence of noise maps having the same dimensions as $z_n(t)$. Here, $\alpha$ determines how close the frames of the sequence remain to $x$, whereas $\beta$ controls the smoothness and rate of change in the generated clip. Note that similarly to the other image manipulation tasks, here as well we can start the animation from different scales so as to obtain different effects. Please see the supplementary video for animation results.

%Pay attention that in this application the generation can be started at different scales $n$. This, as well as changing the parameters $\alpha, \beta$ can control the variability between frames. Please see the attached pptx file for results.

\newpage
%\section{\Large{Additional Results}}
\section{Additional Results}
%We next provide additional experimental results. 
%\newpage
\subsection{Random Samples}
%\newpage

\begin{figure}[h!]
\center
	\includegraphics[width=1\textwidth]{samples1.pdf}
	%\caption{\textbf{Super-resolution.}}
	%\label{fig:SR}
\end{figure}
\vspace{3cm}
\begin{figure}[h!]
\center
	\includegraphics[width=1\textwidth]{samples2.pdf}
	%\caption{\textbf{Super-resolution.}}
	%\label{fig:SR}
\end{figure}
\vspace{3cm}
\begin{figure}[h!]
    \center
	\includegraphics[width=0.8\textwidth]{HR1.pdf}
	%\label{fig:harmonization}
\end{figure}
\begin{figure}[h!]
    \center
	\includegraphics[width=0.75\textwidth]{HR2.pdf}
	%\label{fig:harmonization}
\end{figure}
%\begin{figure*}[h!]
%    \center
%	\includegraphics[width=0.82\textwidth]{HR3.pdf}
	%\label{fig:harmonization}
%\end{figure*}
\begin{figure}[h!]
    \center
	\includegraphics[width=0.8\textwidth]{HR4.pdf}
	%\label{fig:harmonization}
\end{figure}

\newpage
\subsection{Samples at arbitrary dimensions}
%different effect than the task of image retargeting: (i) our resizing is stochastic (\ie volcano) (ii) for expansions, SinGAN generates new image structures (iii) for reduction, we are not restrict to the original image structure.
%\newpage
Using SinGAN, we can generate samples of arbitrary size and aspect ratio. While this is superficially similar to retargeting, the two tasks are distinct. We illustrate this below through comparison to seam carving \cite{avidan2007seam}. In our case, the samples are \emph{random} and are not optimized to maintain salient objects or strong edges. This often leads to plausible configurations that do not appear in the input image. In image retargeting, on the other hand, structures are typically restricted to those appearing in the image, and may deform unrealistically at extreme aspect ratios.

\begin{figure}[h!]
\center
	\includegraphics[width=1\textwidth]{SC3_1.pdf}
	%\caption{\textbf{Generation vs.~retargeting.} Using SinGAN, we can generate samples of arbitrary size and aspect ratio. While superficially similar to retargeting, the two tasks are distinct, as we illustrate here through comparison to seam carving \cite{avidan2007seam}. In our case, the samples are \emph{random} and are not optimized to maintain salient objects or strong edges. This often leads to plausible configurations that do not appear in the input image. In image retargeting, on the other hand, the structures are typically restricted to those appearing in the image.}
	%\label{fig:SR}
\end{figure}
%\vspace{3cm}
\begin{figure}[h!]
\center
	\includegraphics[width=1\textwidth]{SC3_2.pdf}
	%\caption{\textbf{Generation vs.~retargeting.}}
	%\label{fig:SR}
	\vspace{3cm}
\end{figure}

%\newpage
%\subsection{High Resolution Samples}
%\newpage

\subsection{AMT Survey Images}
%\newpage\
%\vspace{-2.5cm}

\begin{figure}[h!]
\center
%\vspace{-2.5cm}
	\includegraphics[width=1\textwidth]{AMT1.pdf}
	%\caption{\textbf{Super-resolution.}}
	%\label{fig:SR}
	\vspace{1.cm}
\end{figure}
%\vspace{3cm}

\begin{figure}[h!]
\center
	\includegraphics[width=1\textwidth]{AMT2.pdf}
	%\caption{\textbf{Super-resolution.}}
	%\label{fig:SR}
	\vspace{1.4cm}
\end{figure}

\begin{figure}[h!]
\center
	\includegraphics[width=1\textwidth]{AMT3.pdf}
	%\caption{\textbf{Super-resolution.}}
	%\label{fig:SR}
	\vspace{1.4cm}
\end{figure}
%\vspace{3cm}

\subsection{Super-resolution \vspace{0.1cm}}
%\newpage
%\vspace{3cm}

\begin{figure}[h!]
%\vspace{0.2cm}
\center
	\includegraphics[width=0.95\textwidth]{SR1.pdf}
	%\caption{\textbf{Super-resolution.}}
	%\label{fig:SR}
	\vspace{0.19cm}
\end{figure}
%\vspace{3cm}

\begin{figure}[h!]
\center
	\includegraphics[width=1\textwidth]{SR2_2.pdf}
	%\caption{\textbf{Super-resolution.}}
	%\label{fig:SR}
	%\vspace{3cm}
\end{figure}
%\vspace{3cm}

%\newpage
\subsection{Harmonization}
%\newpage 

\begin{figure*}[h!]
\center
	\includegraphics[width=1\textwidth]{harmonization_SM.pdf}
	\label{fig:harmonization1}
    %\vspace{3cm}
\end{figure*}

\begin{figure*}[h!]
\center
	\includegraphics[width=1\textwidth]{harmonization_SM2.pdf}
	\label{fig:harmonization2}
    %\vspace{3cm}
\end{figure*}

%\vspace{5cm}

%\begin{figure*}[h!]
%\center
%	\includegraphics[width=1\textwidth]{Figures/harmonization_3.pdf}
%	\label{fig:harmonization}
%\end{figure*}
%\vspace{6cm}
%\begin{figure*}[h!]
%\center
%	\includegraphics[width=1\textwidth]{Figures/harmonization_4.pdf}
%	\label{fig:harmonization}
%\end{figure*}
%\vspace{3cm}

%\newpage
\subsection{Editing}
%\newpage
\begin{figure*}[h!]
\center
	\includegraphics[width=0.87\textwidth]{editing1.pdf}
	%\label{fig:harmonization}
	%\vspace{3cm}
\end{figure*}

%\vspace{3cm}

\newpage
%\begin{figure*}[h!]
%\center
%	\includegraphics[width=0.9\textwidth]{Figures/editing2.pdf}
%	\label{fig:harmonization}
%\end{figure*}
%\vspace{3cm}

%\newpage
\subsection{Paint to Image}
%\newpage
\begin{figure*}[h!]
\center
	\includegraphics[width=0.65\textwidth]{paint_SM.pdf}
	\label{fig:paint}
	%\vspace{3cm}
\end{figure*}

%\vspace{3cm}

%\newpage
\subsection{Experimental Settings}
The tables below report the settings used for each of the results presented in the main text as well as in this supplementary material. For each application, we specify the scale in which the input image was injected and the total number of scales we used for SinGAN's generation pyramid.

\begin{table}[h!]
    \centering
    \begin{tabular}{|c|c|c|}
    \hline
    Image & Injection scale & Total number of scales  \\
    \hline
    Tree (also Fig.~2, main text)& $n = 1$ & $N =9$\\
    Two Dolphins (also Fig.~13, main text)& $n = 3$ & $N = 9$\\
    Single Dolphin & $n = 3$ & $N = 9$\\
    Fox & $n = 2$ & $N = 8$\\
    Airplane & $n = 2$ & $N = 8$\\
    Butterfly & $n = 2$ & $N = 8$\\
    Eagle & $n = 2$ & $N = 8$\\
    Spaceship (also Fig.~13, main text)& $n = 3$ & $N = 8$\\
    Hat & $n = 4$ & $N = 9$\\
    Lemon & $n = 3$ & $N = 7$\\
    Cat & $n = 2$ & $N = 8$\\
    \hline
    \end{tabular}
    \caption{{\bf Harmonization.}}
\end{table}

\begin{table}[h!]
    \centering
    \begin{tabular}{|c|c|c|}
    \hline
    Image & Injection scale & Total number of scales  \\
    \hline
    Rock1 & $n = 5$ & $N = 7$\\
    Rock2 & $n = 5$ & $N = 7$\\
    Rock3 (also Fig.~12, main text)& $n = 5$ & $N = 7$\\
    Tree & $n = 7$ & $N = 9$\\
    Mountain & $n = 4$ & $N = 8$\\
    Red cliff & $n = 5$ & $N = 9$\\
    Hay & $n = 6$ & $N = 9$\\
    \hline
    \end{tabular}
    \caption{{\bf Editing.}}
\end{table}

\begin{table}[h!]
    \centering
    \begin{tabular}{|c|c|c|}
    \hline
    Image & Injection scale & Total number of scales  \\
    \hline
    Balloons1 & $n = 7$ & $N=9$\\
    Balloons2 & $n = 5$ & $N=9$\\
    Starry night & $n = 6$ & $N=8$\\
    Rock & $n = 6$ & $N=8$\\
    Tree & $n = 6$ & $N=8$\\
    Birds & $n = 6$ & $N=7$\\
    View (Fig.~2, main text) & $n = 7$ & $N=8$\\
    Pyramids (Fig.~11, main text)  & $n = 6$ & $N=8$\\
    cows (Fig.~11, main text) & $n = 5$ & $N=7$\\
    \hline
    \end{tabular}
    \caption{{\bf Paint to image.}}
\end{table}

\begin{table}[t]
    \centering
    \begin{tabular}{|c|c|c|c|c|}
    \hline
    Image & Random walk starting scale &  Total number of scales & $\alpha$ & $\beta$  \\
    \hline
    Coral & $n=5$ & $N=7$ & 0.1 &  0.9 \\
    Corals and fish & $n=6$ & $N=8$ & 0.1 &  0.9 \\
    Water  & $n=8$ & $N=8$ & $ 0.1 $ &  $ 0.8 $ \\
    Bush  & $n=6$ & $N=8$ & $ 0.1 $ &  $ 0.9 $ \\
    Trees (slow wind) & $n=6$ & $N=8$ & $0.1 $ &  $0.9 $ \\
    Trees (strong wind) & $n=6$ & $N=8$ & $0.1 $ &  $0.8 $ \\
    Lightning  & $n=7$ & $N=7$ & $ 0.1 $ &  $ 0.9 $ \\
    Fog & $n=5$ & $N=7$ & $ 0.02 $ &  $ 0.95$ \\
    Fire1 & $n=8$ & $N=8$ & $ 0.2 $ &  $ 0.6 $ \\
    %Fire2  & $n=8$ & $N=8$ & $ 0.1 $ &  $ 0.5 $ \\
    Aurora & $n=7$ & $N=8$ & $ 0.1 $ &  $ 0.9 $ \\
    \hline
    \end{tabular}
    \caption{{\bf Single image animation.} See supplementary video.}
\end{table}

%\newpage
