# Supplementary material for: SinGAN: Learning a Generative Model from a Single Natural Image
Source: arXiv:1905.01164 source file (2019-09-04)
Supplement: Supplementary file 2 [file supplementary.tex]

% \paragraph{Optimization}
% At each scale, the weights of the generator and discriminator are initialized to those from the previous trained scale (except for the coarsest scale or when changing the number of kernels, in which cases we use random initialization). We train each scale for 2000 iterations. In each iteration we alternate between 3 gradient steps of the generator and 3 gradient steps of the discriminator. We use Adam \cite{kingma2014adam} with a learning rate of $0.0005$ (decreased by a factor of $0.1$ after $1600$ iterations) and momentum parameters $\beta_1=0.5, \beta_2=0.999$. The weight of the reconstruction loss is $\alpha = 10$, and the weight of the gradient penalty in the WGAN loss is $0.1$. Training takes about $30$ minutes on a 1080TI GPU for an image of size $256\times256$ pixels, and the generation at test time is well under one second per image.
